# Supplementary material for: Anisotropic Agglomerative Adaptive Mean-Shift
Source: arXiv:1411.4102 source file (2014-11-15)
Supplement: Supplementary file 1 [file aaams_supplementary_arxiv.pdf]

# Anisotropic Agglomerative Adaptive Mean-Shift

## Supplementary Material

Rahul Sawhney<sup>1</sup>  
rahul.sawhney@gatech.edu

Henrik I. Christensen<sup>1</sup>  
hic@gatech.edu

Gary R. Bradski<sup>2</sup>  
gbradski@magicleap.com

<sup>1</sup> Institute of Robotics & Intelligent Machines  
Georgia Institute of Technology  
Atlanta, USA

<sup>2</sup> Magic Leap, Inc.  
Dania Beach, USA

We provide a proof of convergence for the case when bandwidths change between Mean Shift iterations, utilizing some of the analysis presented in the References [1, 2, 3, 4].

The proof is over datasets following a normal distribution using a normal kernel under local homoscedasticity. These assumptions are commonly deployed for theoretical analysis of Mean Shift and hold under large sample approximations.  $I$ , is the identity matrix.  $G(x)$ , indicates a normal kernel. Superscript  $\tau$  indicates the current iteration.  $\Sigma_u^\tau$  would then be the updated (symmetric positive definite) bandwidth of cluster  $u$ , at the iteration  $\tau$ .

**Lemma 1 :** *If the true dataset distribution is normal,  $f \sim \mathbf{N}(\mu, \Psi)$ , it follows that the kernel density estimate using a normal kernel under local homoscedasticity, around the trajectory point  $x_{u,u}^\tau \stackrel{\text{def}}{=} u^\tau$ , will also be an asymptotically Gaussian surface given by*

$$p(u^\tau) \sim \mathbf{N}(\mu, \Psi + \Sigma_u^\tau) \quad \langle 1 \rangle$$

**proof:** From analysis in [4]. This can also be seen by noting that the expectation of the density estimate is a convolution of the true density,  $f(x)$ , with the kernel function,  $G(x)$ . Thus, we have  $E[p(x)] = E[f(x) * G(x)]$ . The result ensues since both  $f, G$  are Gaussian functions.

**Lemma 2 :** *The mean shift vector at the cluster/trajectory location  $x_{u,u}^\tau$ , given by  $m(x_{u,u}^\tau) \stackrel{\text{def}}{=} m(u^\tau)$ , would be*

$$m(u^\tau) = \Sigma_u^\tau \frac{\nabla p(u^\tau)}{p(u^\tau)} = -\Sigma_u^\tau (\Psi + \Sigma_u^\tau)^{-1} (u^\tau - \mu) \quad \langle 2 \rangle$$

**proof:** From analysis in [1, 2], by calculating  $\nabla p(u^\tau)$  using Lemma 1, multiplying both sides by  $\Sigma_u^\tau$  and using  $\langle 1 \rangle$ .

**Lemma 3** : Given a symmetric positive semi-definite matrix  $A$  and a symmetric positive definite matrix  $B$ , all eigenvalues of  $AB$  are non-negative and  $AB$  is diagonalizable.

**proof** : We know that  $\text{Spectrum}(AB) = \text{Spectrum}(BA)$ . Thus,  $\text{Spectrum}(AB) = \text{Spectrum}(AB^{1/2}B^{1/2}) = \text{Spectrum}(B^{1/2}AB^{1/2})$ , where  $B^{1/2}$  is the unique, symmetric positive definite, invertible, square root of the symmetric positive definite matrix  $B$ . It follows from *Sylvester's law of inertia* that  $B^{1/2}AB^{1/2}$  will have the same number of positive, zero and negative eigenvalues as  $A$ . Since  $A$  is symmetric positive semi-definite,  $B^{1/2}AB^{1/2}$  and hence  $AB$  will have all eigenvalues as non-negative reals.  $AB$  can be transformed into a symmetric matrix by applying  $B^{1/2}$  as a similarity transformation. Since the resultant symmetric matrix,  $B^{1/2}AB^{1/2}$ , is always diagonalizable, by transitivity,  $AB$  would always be diagonalizable too.

**Proposition 1** : If the trajectory point,  $x_{u,u}^\tau \stackrel{\text{def}}{=} u^\tau$ , lies on a normal distribution,  $N(\mu, \Omega^\tau)$ , the trajectory point,  $x_{u,u}^{\tau+1} \stackrel{\text{def}}{=} u^{\tau+1}$ , resulting due to the next mean shift update, will still follow a normal distribution,  $N(\mu, \Phi^\tau \Omega^\tau \Phi^{\tau T})$  with

$$\Phi^\tau = I - \Sigma_u^\tau (\Psi + \Sigma_u^\tau)^{-1} \quad (3)$$

**proof** : (Similar to analysis in [3]) The updated trajectory point would be

$$u^{\tau+1} = u^\tau + m(u^\tau) \quad (4)$$

Substituting (2) in above, we'll have :

$$\begin{aligned} u^{\tau+1} &= u^\tau - \Sigma_u^\tau (\Psi + \Sigma_u^\tau)^{-1} (u^\tau - \mu) \\ &= (I - \Sigma_u^\tau (\Psi + \Sigma_u^\tau)^{-1}) u^\tau + \Sigma_u^\tau (\Psi + \Sigma_u^\tau)^{-1} \mu \\ &\xrightarrow{\text{yields}} u^{\tau+1} = \Phi^\tau u^\tau + \Sigma_u^\tau (\Psi + \Sigma_u^\tau)^{-1} \mu \end{aligned} \quad (5)$$

The second term in (5) is a constant vector, while the first term is a scaled Gaussian random variable. Thus  $u^{\tau+1}$  is basically a linear transformation of  $u^\tau$ . It follows that when  $u^\tau \sim N(\mu, \Omega^\tau)$ ,  $u^{\tau+1}$  will also follow a linearly transformed normal distribution specified as :

$$\begin{aligned} u^{\tau+1} &\sim N(\Phi^\tau \mu + \Sigma_u^\tau (\Psi + \Sigma_u^\tau)^{-1} \mu, \Phi^\tau \Omega^\tau \Phi^{\tau T}) \\ &\sim N((\Phi^\tau + \Sigma_u^\tau (\Psi + \Sigma_u^\tau)^{-1}) \mu, \Phi^\tau \Omega^\tau \Phi^{\tau T}) \\ &\xrightarrow{\text{yields}} u^{\tau+1} \sim N(\mu, \Phi^\tau \Omega^\tau \Phi^{\tau T}) \end{aligned} \quad (6)$$

Since the trajectory originates from  $u^{\tau=0} \stackrel{\text{def}}{=} x_{u,u}^{\tau=0} \stackrel{\text{def}}{=} x_{u,u}$ , which is normally distributed (with  $\Omega^{\tau=0} = \Psi$ ) - all trajectory points follow normal distributions,  $u^{\tau+1} \sim N(\mu, \Phi^\tau \Omega^\tau \Phi^{\tau T})$ ,  $\forall \tau$  - with means coincident with the true distribution's mode,  $\mu$ .

**Proposition 2** :  $|\Phi^\tau| < 1, \forall \tau$

**proof** : (Similar to analysis in [3]) We have from (3)

$$\begin{aligned} \Phi^\tau &= \mathbf{I} - \Sigma_u^\tau (\Psi + \Sigma_u^\tau)^{-1} \\ \xrightarrow{\text{yields}} \Phi^\tau &= \mathbf{I} - (\Psi(\Sigma_u^\tau)^{-1} + \mathbf{I})^{-1} \end{aligned} \quad (7)$$

Since  $\Psi$  is symmetric positive semi-definite and  $(\Sigma_u^\tau)^{-1}$  is symmetric positive definite, from Lemma 3, their product is diagonalizable and can be eigen-decomposed. We have then  $\Psi(\Sigma_u^\tau)^{-1} = \mathbf{Q}^\tau \Lambda^\tau \mathbf{Q}^{\tau T}$ , where  $\Lambda^\tau = \text{diag}(\lambda_1, \lambda_2, \lambda_3, \dots)$  is the diagonal matrix of eigenvalues which are all non-negative (Lemma 3) and  $\mathbf{Q}^\tau$  is the orthonormal matrix of eigenvectors.

Using Woodbury inversion lemma on (7), we'll have :

$$\Phi^\tau = \mathbf{I} - (\mathbf{Q}^\tau \Lambda^\tau \mathbf{Q}^{\tau T} + \mathbf{I})^{-1} = \mathbf{Q}^\tau (\mathbf{I} - (\mathbf{I} + \Lambda^\tau)^{-1}) \mathbf{Q}^{\tau T} \quad (8)$$

Applying norms on both sides, and under orthonormality of  $\mathbf{Q}^\tau$  :

$$\begin{aligned} |\Phi^\tau| &= |\mathbf{Q}^\tau (\mathbf{I} - (\mathbf{I} + \Lambda^\tau)^{-1}) \mathbf{Q}^{\tau T}| \\ &= |(\mathbf{I} - (\mathbf{I} + \Lambda^\tau)^{-1})| \\ \xrightarrow{\text{yields}} |\Phi^\tau| &= \left| \text{diag} \left( \frac{\lambda_1}{1 + \lambda_1}, \frac{\lambda_2}{1 + \lambda_2}, \frac{\lambda_3}{1 + \lambda_3}, \dots \right) \right| \end{aligned} \quad (9)$$

Since all eigenvalues are non-negative, all the diagonal entries, and hence their product is less than one. Thus,  $|\Phi^\tau| < 1$  will always hold true as long as the bandwidth matrix,  $\Sigma_u^\tau$ , remains symmetric positive definite. Moreover, if  $\Psi$  is symmetric positive definite, *i.e.* does not have any zero eigenvalues,  $|\Phi^\tau| > 0$  always. To maintain clarity in exposition, we assume this to be the case for Propositions 3 & 4. If  $f$  does have some degenerate subspaces, similar analysis over the non-degenerate subspaces will result in equivalent conclusions.

**Proposition 3** : Each mean shift update moves the trajectory closer to  $\mu$ , the true distribution's mode.

**proof** : Subtracting  $\mu$  from both sides in (4) and substituting (2), we'll have

$$\begin{aligned} u^{\tau+1} - \mu &= u^\tau - \Sigma_u^\tau (\Psi + \Sigma_u^\tau)^{-1} (u^\tau - \mu) - \mu \\ &= (u^\tau - \mu) (\mathbf{I} - \Sigma_u^\tau (\Psi + \Sigma_u^\tau)^{-1}) \end{aligned}$$

From (3) then :

$$\xrightarrow{\text{yields}} u^{\tau+1} - \mu = (u^\tau - \mu) \Phi^\tau \quad (10)$$

Taking norm on both sides :

$$|u^{\tau+1} - \mu| = |(u^\tau - \mu) \Phi^\tau|$$

Since  $|M_1 M_2| \leq |M_1| |M_2|$ , we'll have then :

$$|u^{\tau+1} - \mu| \leq |u^\tau - \mu| |\Phi^\tau| \quad (11)$$

Therefore, until convergence *i.e.*  $|u^\tau - \mu| \neq 0$ ,

$$\text{Equation (11)} \xrightarrow{\forall \tau, \text{ implies}} |u^{\tau+1} - \mu| < |u^\tau - \mu|, \text{ since } |\Phi^\tau| < 1, \forall \tau$$

The cluster trajectory will hence move closer to the true distribution mode in every iteration.

**Proposition 4 :** *The trajectory,  $u^\tau$ , will asymptotically converge to the true distribution mode,  $\mu$*

**proof:** We have from (11)

$$|u^{\tau+1} - \mu| \leq |u^\tau - \mu| |\Phi^\tau|$$

Applying (11) recursively, gets us

$$\begin{aligned} |u^{\tau+1} - \mu| &\leq |u^{\tau-1} - \mu| |\Phi^{\tau-1}| |\Phi^\tau| \\ &\leq |u^{\tau-2} - \mu| |\Phi^{\tau-2}| |\Phi^{\tau-1}| |\Phi^\tau| \\ &\dots \dots \dots \\ &\dots \dots \dots \\ &\leq |u^{\tau=0} - \mu| \prod_{\omega=0}^{\tau} |\Phi^\omega| \end{aligned} \quad (12)$$

Since  $u^{\tau=0} \stackrel{\text{def}}{=} x_{u,u}$ , and the norms by definition are non-negative, we'll have :

$$0 \leq |u^{\tau+1} - \mu| \leq |x_{u,u} - \mu| \prod_{\omega=0}^{\tau} |\Phi^\omega| \quad (13)$$

Since,  $|x_{u,u} - \mu| < \infty$  &  $|\Phi^\omega| < 1, \forall \omega$ , we have :

$$\lim_{\tau \rightarrow \infty} |x_{u,u} - \mu| \prod_{\omega=0}^{\tau} |\Phi^\omega| = 0 \quad (14)$$

By *Sandwich theorem of limits* then,

$$\lim_{\tau \rightarrow \infty} |u^{\tau+1} - \mu| = 0 \quad (15)$$

*Thus, the cluster trajectory will eventually converge to the true distribution mode,  $\mu$ .*

---

## References

- [1] Comaniciu, D., & Meer, P. (2002). Mean shift: A robust approach toward feature space analysis. *Pattern Analysis and Machine Intelligence, IEEE Transactions on*, 24(5), 603-619.
- [2] Comaniciu, D. (2003). An algorithm for data-driven bandwidth selection. *Pattern Analysis and Machine Intelligence, IEEE Transactions on*, 25(2), 281-288.
- [3] Zhang, K., Kwok, J. T., & Tang, M. (2006). Accelerated convergence using dynamic mean shift. In *Computer Vision—ECCV 2006* (pp. 257-268). Springer Berlin Heidelberg.
- [4] Stoker, T. M. (1993). Smoothing bias in density derivative estimation. *Journal of the American Statistical Association*, 88(423), 855-863.
